# Supplementary material for: "Knees" in lithium-ion battery aging trajectories
Source: arXiv:2201.02891 ancillary file (2022-01-08)
Supplement: Supplementary file 1 [file SI.pdf]

## Supplementary Information for

# "Knees" in lithium-ion battery aging trajectories


Peter M. Attia,*,† Alexander Bills,‡ Ferran Brosa Planella,¶ Philipp Dechent,§ Gonçalo dos Reis,‖ Matthieu Dubarry,⊥ Paul Gasper,# Richard Gilchrist,@ Samuel Greenbank,△ David Howey,▽ Ouyang Liu,†† Edwin Khoo,†† Yuliya Preger,‡‡ Abhishek Soni,¶¶ Shashank Sripad,‡ Anna G. Stefanopoulou,§§ and Valentin Sulzer§§

†*Department of Materials Science and Engineering, Stanford University, Stanford, CA, USA*

‡*Department of Mechanical Engineering, Carnegie Mellon University, Pittsburgh, PA, USA*

¶*WMG, University of Warwick, Coventry, UK, and Faraday Institution, Harwell, UK*

§*Institute for Power Electronics and Electrical Drives (ISEA), RWTH Aachen University, Aachen, Germany*

‖*School of Mathematics, University of Edinburgh, Edinburgh, UK and Centro de Matemática e Aplicações (CMA), FCT, UNL, Caparica, Portugal*

⊥*Hawaii Natural Energy Institute, University of Hawaii at Manoa, Honolulu, HI, USA*

#*National Renewable Energy Laboratory, Golden, CO, USA*

@*School of Mathematics, University of Edinburgh, Edinburgh, UK*

△*Department of Engineering Science, University of Oxford, Oxford, UK*

▽*Department of Engineering Science, University of Oxford, Oxford, UK, and Faraday Institution, Harwell, UK*

††*Institute for Infocomm Research, Agency for Science, Technology, and Research (A*STAR), Connexis, Singapore*

‡‡*Sandia National Laboratories, Albuquerque, NM, USA*

¶¶*Department of Mechanical Engineering, University of Cincinnati, Cincinnati, OH, USA*

§§*Department of Mechanical Engineering, University of Michigan, Ann Arbor, MI, USA*

E-mail: peter.m.attia@gmail.com

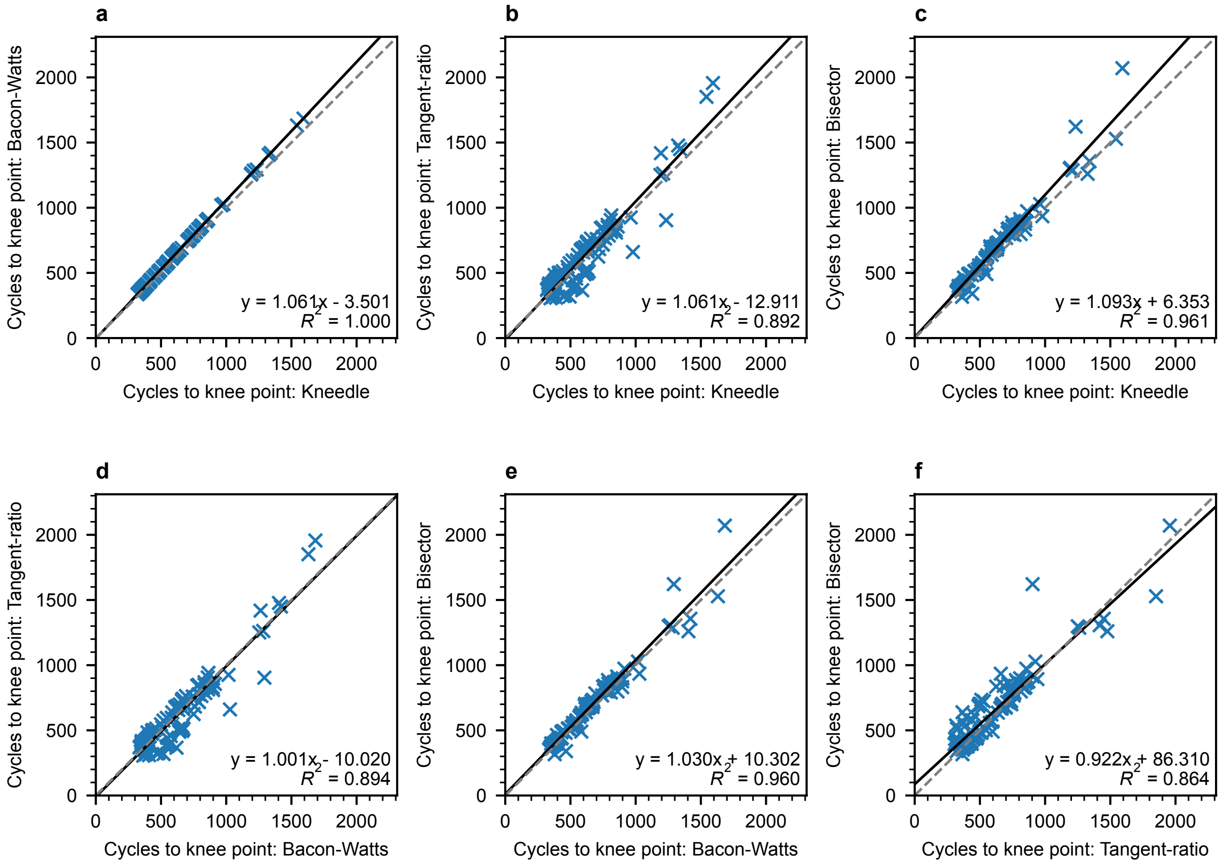


Figure S1. Linear regressions comparing various knee point estimation algorithms for the capacity curves of the Severson et al.[1] dataset (except the quantile regression method[2]). We mention that the true knee point has no "ground truth". The results from the Kneedle[3] and Bacon-Watts[4] methods are highly correlated with each other ($R^2 \approx 1$). The bisector[5] is also highly correlated with these two methods ($R^2 \approx 0.96$). The tangent-ratio method[6] has the poorest correlation with the others.

.

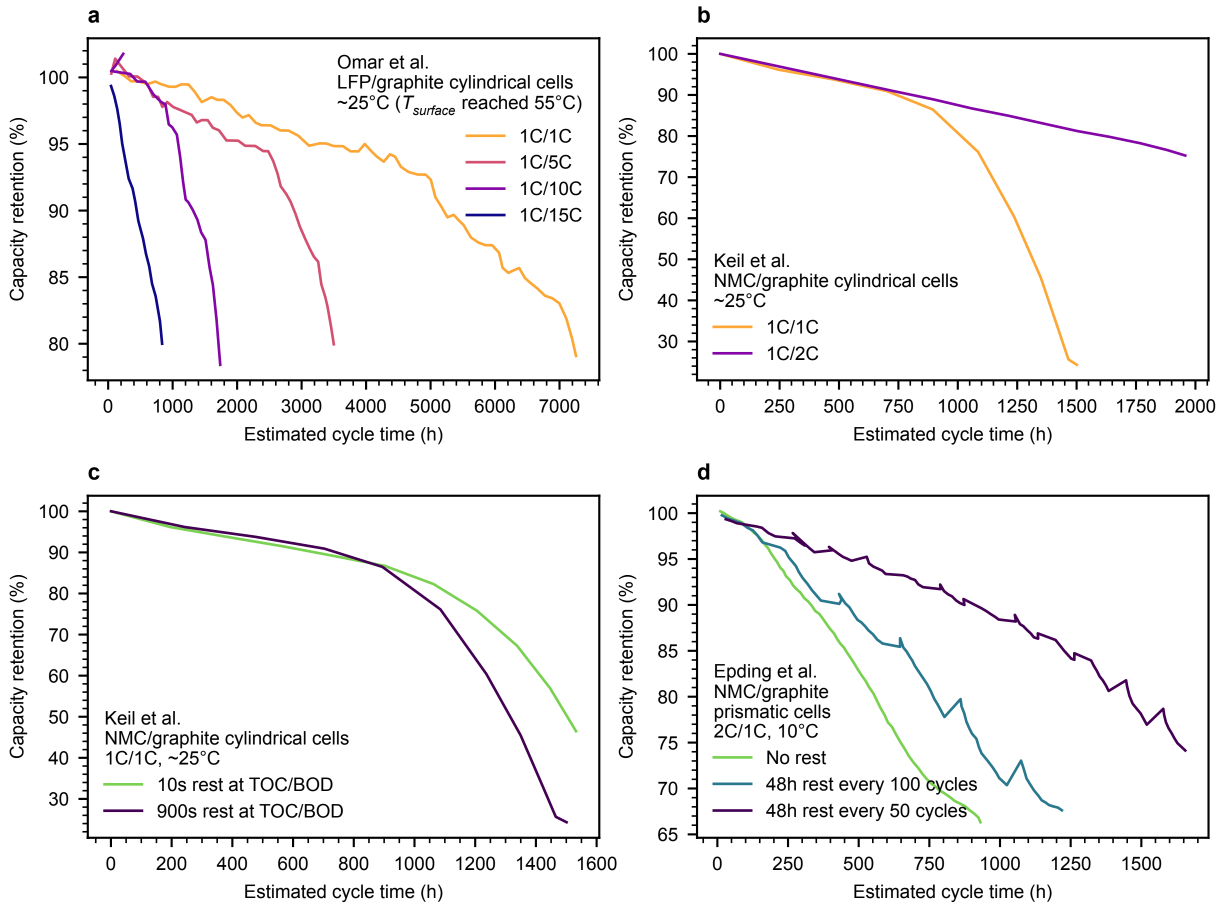


Figure S2. Mixed effects of discharge rate and rest time on knee onset, depending on the testing conditions. Data replotted from Figure 20 with a time-based $x$ axis (estimated from C rates). Raw data from the corresponding studies were not available, so the cycle times were estimated from the given C rates and rest times. While the trends in discharge rate and rest time influence on knee onset are largely the same as in the cycle-based figure (Figure 20), the change from Figure 20c to Figure S2c suggests that much of the reason that longer rest times at top-of-charge and bottom-of-discharge decrease cycle life (at least in this study) is calendar aging, not greater degradation at the voltage extremes. Thus, the use of a cycle-based $x$ axis may obscure calendar aging phenomena. (a) Higher discharge rate can accelerate knee onset. Adapted from Figure 8 of Omar et al.[7] Note that while the environmental test temperature was ∼25°C, the temperature at the surface reached as high as 55°C for the high rate discharge tests. (b) Lower discharge rate can accelerate knee onset. Adapted from Figure 2a of Keil et al.[8] (c) Longer rest time can accelerate knee onset. Adapted from Figure 2a of Keil et al.[8] (d) Shorter rest time can accelerate knee onset. Adapted from Figure 1a of Epding et al.[9]

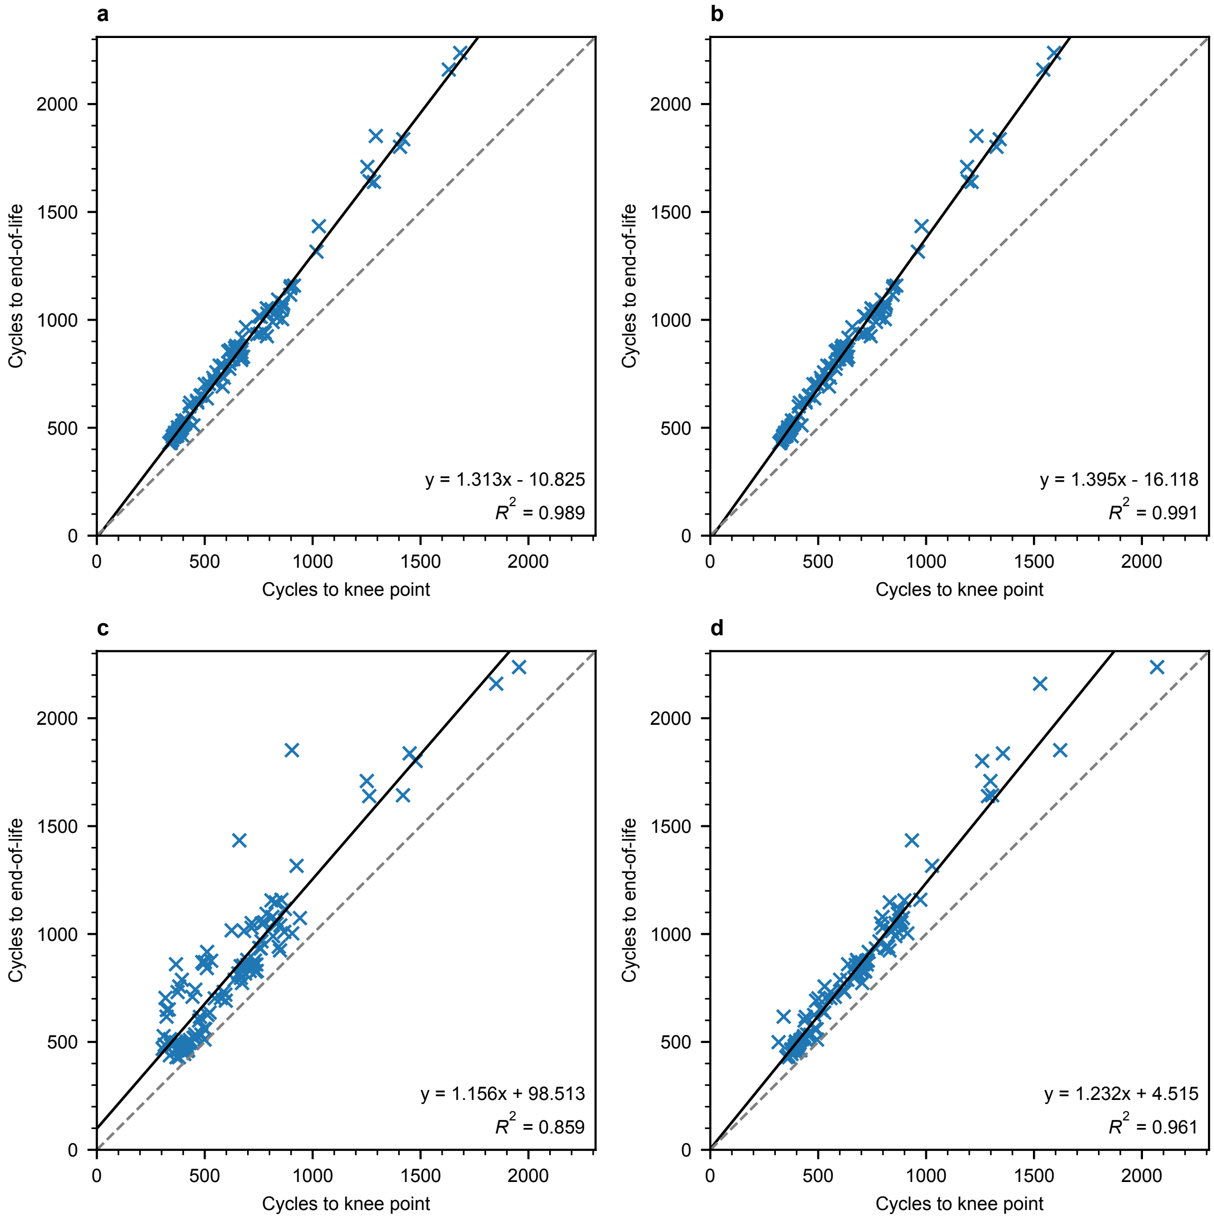


Figure S3. Linear relationship between identified knees and end-of-life (EOL) per knee identification algorithm over the Severson et al.[1] dataset. (a) Bacon-Watts[4], (b) Kneedle[3], (c) Tangent-ratio[6], (d) Bisector[5]. We mention that there is no "ground truth" for the true knee. For the Bacon-Watts and Kneedle identified knees, the linear regression holds with a goodness-of-fit of $R^2 \approx 99\%$ (and reduced variance between fit and residuals). With this metric, close by is the bisector[5] with a correlation of $R^2 \approx 0.96$. The tangent-ratio[6] identified knees show a higher fit-to-residuals variability ($R^2 \approx 0.86$).

.

**Table SI. Summary of references used to generate Figure 22 in the main manuscript. The data was obtained extracted via direct access to the corresponding databases when possible[1,10–13] or via *WebPlotDigitizer*.[14]**

| Reference | Cell Description | Number of cells | Capacity curve references |
|---|---|---|---|
| Aiken et al.[15] 2020 | Lab-made pouch NMC/Gr | 4 | Fig 3d 0.8M, 1.2M;<br>Fig 10a: `red circle' and `blue circle' |
| Baumhöfer et al.[10] 2014 | Sanyo UR18650E NMC/Gr | 48 | Database access |
| Broussely et al.[16] 2005 | Saft VLE NCA/Gr | 2 | Fig 2 red and green |
| Burns et al.[17] 2015 | Panasonic 18650 NCA/Gr | 2 | Fig1b circles and squares |
| Coron et al.[18] 2020 | Commercial 18650 NMC+LMO/Gr<br>Commercial 18650 NMC/Gr | 5 | Fig 1c: `red crosses', `red squares',<br>`blue crosses', `blue squares' and `blue circles' |
| Diao et al.[11] 2019 | Pouch LCO/Gr | 34 | Database access |
| Epding et al.[9] 2019 | Commercial prismatic NMC/Gr | 3 | Fig 1a black and green; Fig 7a black cell 2 |
| Keil et al.[19] 2016 | a) Sanyo UR18650SA LMO+NMC/Gr<br>b) Sony US18650VT1 LMO+LCO/Gr<br>c) A123 APR18650M1A LFP/Gr | 5 | Fig 8c 3A CCCV +50mV (C); Fig 10a 1A CCCV (A);<br>Fig 10a 1A CCCV (A); Fig 10b 3A CCCV (B);<br>Fig 10c 5A CCCV (C) |
| Keil et al.[8] 2019 | Cylindrical NMC/Gr | 6 | Fig 2a procedure 1 and 2; Fig 8a procedure 1 100 SOC;<br>Fig 8a procedure 1 0 SOC; Fig 8a procedure 2 100 SOC;<br>Fig 8a procedure 2 0 SOC |
| Klett et al.[20] 2014 | Commercial 26650 LFP/Gr | 1 | Figure 2a CCC |
| Petzl et al.[21] 2015 | Commercial 26650 LFP/Gr | 3 | Fig 1a blue, red, black |
| Schuster et al.[22] 2015 | E-One Moli Energy IHR18650A NMC/Gr | 15 | Fig 1a; Fig 4a 1.30V (CCCV) (A); Fig 4a 1.20V (CCCV) (A);<br>Fig 4a 1.20V (CC) (A); Fig 4a 0.94V (CC) (A);<br>Fig 6a 0.5C/0.5C (A); Fig 6a 1.0C/0.5C (A); Fig 6a 0.5C/1.0C (A);<br>Fig 9 1.20 V (CC); Fig 9 1.20 V (CCCV); Fig 9 1.20 V (2CCCV);<br>Fig 10a 35 C(deltaV down) (A); Fig 10a 35 C(deltaV up) (A);<br>Fig 10a 50 C(deltaV up) (A); Fig 10a 25 C(deltaV up) (A); |
| Severson et al.[1] 2019 | A123 APR18650M1A LFP/Gr | 120 | Database access |
| Willenberg et al.[12] 2020 | Samsung INR18650 35E NCA/Gr+Si | 4 | Database access |

# References


(1) Severson, K. A.; Attia, P. M.; Jin, N.; Perkins, N.; Jiang, B.; Yang, Z.; Chen, M. H.; Aykol, M.; Herring, P. K.; Fraggedakis, D. et al. Data-driven prediction of battery cycle life before capacity degradation. *Nature Energy* **2019**, *4*, 383–391.

(2) Zhang, Y.; Tang, Q.; Zhang, Y.; Wang, J.; Stimming, U.; Lee, A. A. Identifying degradation patterns of lithium ion batteries from impedance spectroscopy using machine learning. *Nature Communications* **2020**, *11*, 1706.

(3) Satopaa, V.; Albrecht, J.; Irwin, D.; Raghavan, B. Finding a "Kneedle" in a Haystack: Detecting Knee Points in System Behavior. 2011 31st International Conference on Distributed Computing Systems Workshops. 2011; pp 166–171, ISSN: 2332-5666.

(4) Fermín-Cueto, P.; McTurk, E.; Allerhand, M.; Medina-Lopez, E.; Anjos, M. F.; Sylvester, J.; dos Reis, G. Identification and machine learning prediction of knee-point and knee-onset in capacity degradation curves of lithium-ion cells. *Energy and AI* **2020**, *1*, 100006.

(5) Greenbank, S.; Howey, D. Automated feature extraction and selection for data-driven models of rapid battery capacity fade and end of life. *IEEE Transactions on Industrial Informatics* **2021**,

(6) Diao, W.; Saxena, S.; Han, B.; Pecht, M. Algorithm to Determine the Knee Point on Capacity Fade Curves of Lithium-Ion Cells. *Energies* **2019**, *12*, 2910.

(7) Omar, N.; Monem, M. A.; Firouz, Y.; Salminen, J.; Smekens, J.; Hegazy, O.; Gaulous, H.; Mulder, G.; Van den Bossche, P.; Coosemans, T. et al. Lithium iron phosphate based battery – Assessment of the aging parameters and development of cycle life model. *Applied Energy* **2014**, *113*, 1575–1585.

(8) Keil, J.; Paul, N.; Baran, V.; Keil, P.; Gilles, R.; Jossen, A. Linear and Nonlinear Aging of Lithium-Ion Cells Investigated by Electrochemical Analysis and In-Situ Neutron Diffraction. *Journal of The Electrochemical Society* **2019**, *166*, A3908–A3917.

(9) Epding, B.; Rumberg, B.; Jahnke, H.; Stradtmann, I.; Kwade, A. Investigation of significant capacity recovery effects due to long rest periods during high current cyclic aging tests in automotive lithium ion cells and their influence on lifetime. *Journal of Energy Storage* **2019**, *22*, 249–256.

(10) Baumhöfer, T.; Brühl, M.; Rothgang, S.; Sauer, D. U. Production caused variation in capacity aging trend and correlation to initial cell performance. *Journal of Power Sources* **2014**, *247*, 332–338.

(11) Diao, W.; Saxena, S.; Pecht, M. Accelerated cycle life testing and capacity degradation modeling of LiCoO2-graphite cells. *Journal of Power Sources* **2019**, *435*, 226830.

(12) Willenberg, L. K.; Dechent, P.; Fuchs, G.; Sauer, D. U.; Figgemeier, E. High-Precision Monitoring of Volume Change of Commercial Lithium-Ion Batteries by Using Strain Gauges. *Sustainability* **2020**, *12*, 557.

(13) Attia, P. M.; Grover, A.; Jin, N.; Severson, K. A.; Markov, T. M.; Liao, Y.-H.; Chen, M. H.; Cheong, B.; Perkins, N.; Yang, Z. et al. Closed-loop optimization of fast-charging protocols for batteries with machine learning. *Nature* **2020**, *578*, 397–402.

(14) Rohatgi, A. Webplotdigitizer: Version 4.5. 2021; `https://automeris.io/WebPlotDigitizer`.

(15) Aiken, C. P.; Harlow, J. E.; Tingley, R.; Hynes, T.; Logan, E. R.; Glazier, S. L.; Keefe, A. S.; Dahn, J. R. Accelerated Failure in Li[Ni0.5Mn0.3Co0.2]O2/Graphite Pouch Cells Due to Low LiPF6 Concentration and Extended Time at High Voltage. *Journal of The Electrochemical Society* **2020**, *167*, 130541, Publisher: The Electrochemical Society.

(16) Broussely, M.; Biensan, P.; Bonhomme, F.; Blanchard, P.; Herreyre, S.; Nechev, K.; Staniewicz, R. Main aging mechanisms in Li ion batteries. *Journal of Power Sources* **2005**, *146*, 90–96.

(17) Burns, J. C.; Stevens, D. A.; Dahn, J. R. In-Situ Detection of Lithium Plating Using High Precision Coulometry. *Journal of The Electrochemical Society* **2015**, *162*, A959–A964.

(18) Coron, E.; Geniès, S.; Cugnet, M.; Thivel, P. X. Impact of Lithium-Ion Cell Condition on Its Second Life Viability. *Journal of The Electrochemical Society* **2020**, *167*, 110556.

(19) Keil, P.; Jossen, A. Charging protocols for lithium-ion batteries and their impact on cycle life—An experimental study with different 18650 high-power cells. *Journal of Energy Storage* **2016**, *6*, 125–141.

(20) Klett, M.; Eriksson, R.; Groot, J.; Svens, P.; Ciosek Högström, K.; Lindström, R. W.; Berg, H.; Gustafson, T.; Lindbergh, G.; Edström, K. Non-uniform aging of cycled commercial LiFePO4//graphite cylindrical cells revealed by post-mortem analysis. *Journal of Power Sources* **2014**, *257*, 126–137.

(21) Petzl, M.; Kasper, M.; Danzer, M. A. Lithium plating in a commercial lithium-ion battery – A low-temperature aging study. *Journal of Power Sources* **2015**, *275*, 799–807.

(22) Schuster, S. F.; Bach, T.; Fleder, E.; Müller, J.; Brand, M.; Sextl, G.; Jossen, A. Nonlinear aging characteristics of lithium-ion cells under different operational conditions. *Journal of Energy Storage* **2015**, *1*, 44–53.
